# Supplementary material for: Electronic structure of $\boldsymbol{\alpha}$-RuCl$_3$ by fixed-node and fixed-phase diffusion Monte Carlo methods
Source: arXiv:2203.15949 ancillary file (2022-08-15)
Supplement: Supplementary file 1 [file RuCl3_supplemental.pdf]

# Supplemental Material for “ Electronic structure of $\alpha$ -RuCl<sub>3</sub> by fixed-node and fixed-phase diffusion Monte Carlo methods ”

Abdulgani Annaberdiyev<sup>1,3</sup>, Cody A. Melton<sup>2</sup>, Guangming Wang<sup>1</sup>, and Lubos Mitas<sup>1</sup>

1) *Department of Physics, North Carolina State University,  
Raleigh, North Carolina 27695-8202, USA*

2) *Sandia National Laboratories,  
Albuquerque, New Mexico 87123, USA*  
and

3) *Center for Nanophase Materials Sciences Division,  
Oak Ridge National Laboratory,  
Oak Ridge, Tennessee 37831, USA*

The Supplemental Material provides additional data regarding the presented calculations. Section I provides data demonstrating the convergence for SCF plane-wave kinetic energy cut-off, SCF  $k$ -mesh, QMC orbital mesh factor, and simulation box size for atoms. Section II provides QMC total, kinetic, and potential energies for various trial wave functions in the selected supercell sizes. In Section III, atomic and solid energies are provided which were used in calculating the cohesive energies. Section IV provides detailed data for QMC nodal optimization calculations. In Section V, all employed supercells are visualized. Section VI provides the solid geometry used in this work. More detailed explanations are provided in the captions of each Table and Figure.

## I. SCF AND ORBITAL CONVERGENCE

TABLE 1: Quantum Espresso SCF kinetic energy cutoff convergence for ZZ phase.  $\Gamma$ -centered  $[2 \times 2 \times 2]$   $k$ -mesh in the conventional cell. DFT+ $U$ (3.0 eV). 400 Ry was used in the main article.

| Ecut [Ry] | Total Energy [Ha] | $\Gamma \rightarrow \Gamma$ gap [eV] |
|-----------|-------------------|--------------------------------------|
| 100       | -558.008320       | 1.6548                               |
| 200       | -558.337787       | 1.6583                               |
| 300       | -558.361104       | 1.6593                               |
| 400       | -558.363409       | 1.6584                               |
| 500       | -558.363660       | 1.6593                               |
| 600       | -558.363697       | 1.6577                               |

TABLE 2: Quantum Espresso SCF  $k$ -mesh convergence for ZZ phase. Ecut = 200 Ry. Meshes are  $\Gamma$ -centered and correspond to the conventional cell. DFT+ $U$ (3.0 eV).  $\Gamma$ -centered  $[2 \times 2 \times 2]$   $k$ -mesh in the conventional cell was used in the main article.

| $k$ -mesh               | Total Energy [Ha] | $\Gamma \rightarrow \Gamma$ gap [eV] |
|-------------------------|-------------------|--------------------------------------|
| $[1 \times 1 \times 1]$ | -558.333662       | 1.6241                               |
| $[2 \times 2 \times 2]$ | -558.337787       | 1.6583                               |
| $[3 \times 3 \times 3]$ | -558.337909       | 1.6595                               |
| $[4 \times 4 \times 4]$ | -558.337928       | 1.6593                               |
| $[5 \times 5 \times 5]$ | -558.337922       | 1.6603                               |

TABLE 3: VMC/(PBE+ $U$  = 2.5 eV) spline mesh convergence for the ZZ phase. Energies are shown in [Ha]. A minimum of 0.6 mesh factor was used in the main article.

| Mesh factor | Total Energy | Kinetic Energy | Total Variance |
|-------------|--------------|----------------|----------------|
| 1.0         | -558.3296(5) | 209.265(6)     | 5.84(1)        |
| 0.9         | -558.3290(5) | 209.265(5)     | 5.852(5)       |
| 0.8         | -558.3293(6) | 209.275(5)     | 5.870(5)       |
| 0.7         | -558.3294(4) | 209.267(5)     | 5.95(2)        |
| 0.6         | -558.3297(5) | 209.265(4)     | 6.046(6)       |
| 0.5         | -558.3287(4) | 209.237(8)     | 6.445(6)       |
| 0.4         | -558.3211(5) | 209.167(5)     | 7.90(1)        |

TABLE 4: Effect of fixed  $ns$  in DFT+ $U$  on energies ( $ns$  is the atomic density appearing in the Hubbard term).  $ns$  values are fixed from the AREP run. Ru atom in a box ( $L = 25.5$  bohr) is used with  $U = 2$  eV. The manuscript used fixed  $ns$  calculations to be able to converge solid calculations.

| Run type     | Energy [Ry]   | Gap [eV] |
|--------------|---------------|----------|
| fixed        | -189.01219328 | 1.4912   |
| released     | -189.01315390 | 1.4892   |
| from scratch | -189.01315175 | 1.4883   |

TABLE 5: Effect of the box size for simulating isolated atoms. Cl atom in a box ( $L \times L \times L$ ) is used with plain PBE.

| $L$ [Angs] | PBE En. [Ry] | PBE Gap [eV] | DMC En. [Ha]  |
|------------|--------------|--------------|---------------|
| 5.0        | -29.77091806 | 0.5437       |               |
| 7.5        | -29.79079351 | 0.5354       |               |
| 10.0       | -29.79125372 | 0.5404       |               |
| 13.5       | -29.79127412 | 0.5395       | -14.9208(1)   |
| 20.0       | -29.79127422 | 0.5383       | -14.9195(2)   |
| 25.0       | -29.79127444 | 0.5383       | -14.91950(15) |

## II. QMC ENERGIES

### A. QMC Energies using PBE0(15%) AREP Trial Wave Function

TABLE 6: QMC total energies [Ha] for various supercell sizes.  $n$  denotes the number of  $\text{RuCl}_3$  chemical formula units in a supercell.  $[0.02, 0.005]$   $\text{Ha}^{-1}$  timestep extrapolation and T-moves were used for DMC.

| State          | Method | $n = 4$        | $n = 16$        | $n = 32$       |
|----------------|--------|----------------|-----------------|----------------|
| GS             | VMC    | -558.33977(70) | -2233.89428(70) | -4467.6396(38) |
| GS             | DMC    | -558.90929(87) | -2235.2058(12)  | -4470.1979(30) |
| $\Gamma\Gamma$ | VMC    | -558.29071(67) | -2233.80978(32) | -4467.5263(30) |
| $\Gamma\Gamma$ | DMC    | -558.8837(13)  | -2235.1385(14)  | -4470.1063(33) |
| CA             | VMC    | -558.49404(60) | -2234.0549(24)  | -4467.7857(32) |
| CA             | DMC    | -559.09089(87) | -2235.3769(26)  | -4470.3721(50) |
| AN             | VMC    | -558.07624(74) | -2233.63546(70) | -4467.3690(39) |
| AN             | DMC    | -558.6694(10)  | -2234.9648(30)  | -4469.9306(29) |

TABLE 7: QMC total energies per  $n$  [Ha] for various supercell sizes.  $n$  denotes the number of  $\text{RuCl}_3$  chemical formula units in a supercell.  $[0.02, 0.005]$   $\text{Ha}^{-1}$  timestep extrapolation and T-moves were used for DMC.

| State          | Method | $n = 4$      | $n = 16$      | $n = 32$      | $\text{TDL}_{16 \rightarrow 32}$ |
|----------------|--------|--------------|---------------|---------------|----------------------------------|
| GS             | VMC    | -139.5849(2) | -139.61839(4) | -139.6137(1)  | -139.6091(2)                     |
| GS             | DMC    | -139.7273(2) | -139.70036(7) | -139.69368(9) | -139.6870(2)                     |
| $\Gamma\Gamma$ | VMC    | -139.5727(2) | -139.61311(2) | -139.61020(9) | -139.6073(2)                     |
| $\Gamma\Gamma$ | DMC    | -139.7209(3) | -139.69616(9) | -139.6908(1)  | -139.6855(2)                     |
| CA             | VMC    | -139.6235(1) | -139.6284(1)  | -139.6183(1)  | -139.6082(3)                     |
| CA             | DMC    | -139.7727(2) | -139.7111(2)  | -139.6991(2)  | -139.6872(4)                     |
| AN             | VMC    | -139.5191(2) | -139.60222(4) | -139.6053(1)  | -139.6083(2)                     |
| AN             | DMC    | -139.6673(3) | -139.6853(2)  | -139.68533(9) | -139.6854(3)                     |

TABLE 8: QMC kinetic energies per  $n$  [Ha] for various supercell sizes.  $n$  denotes the number of  $\text{RuCl}_3$  chemical formula units in a supercell.  $[0.02, 0.005]$   $\text{Ha}^{-1}$  timestep extrapolation and T-moves were used for DMC.

| State          | Method | $n = 4$   | $n = 16$   | $n = 32$  | $\text{TDL}_{16 \rightarrow 32}$ |
|----------------|--------|-----------|------------|-----------|----------------------------------|
| GS             | VMC    | 52.287(2) | 52.225(2)  | 52.28(1)  | 52.33(3)                         |
| GS             | DMC    | 52.274(2) | 52.252(3)  | 52.252(2) | 52.251(5)                        |
| $\Gamma\Gamma$ | VMC    | 52.248(2) | 52.2161(9) | 52.27(1)  | 52.33(3)                         |
| $\Gamma\Gamma$ | DMC    | 52.240(4) | 52.240(2)  | 52.249(2) | 52.258(5)                        |
| CA             | VMC    | 51.982(3) | 52.121(1)  | 52.186(1) | 52.252(2)                        |
| CA             | DMC    | 51.973(3) | 52.153(3)  | 52.210(3) | 52.267(7)                        |
| AN             | VMC    | 52.555(2) | 52.3099(9) | 52.32(1)  | 52.32(3)                         |
| AN             | DMC    | 52.544(4) | 52.319(1)  | 52.293(2) | 52.266(4)                        |

TABLE 9: QMC potential energies per  $n$  [Ha] for various supercell sizes.  $n$  denotes the number of  $\text{RuCl}_3$  chemical formula units in a supercell.  $[0.02, 0.005]$   $\text{Ha}^{-1}$  timestep extrapolation and T-moves were used for DMC.

| State          | Method | $n = 4$     | $n = 16$     | $n = 32$    | $\text{TDL}_{16 \rightarrow 32}$ |
|----------------|--------|-------------|--------------|-------------|----------------------------------|
| GS             | VMC    | -191.872(2) | -191.844(2)  | -191.89(1)  | -191.93(3)                       |
| GS             | DMC    | -192.001(2) | -191.952(3)  | -191.945(2) | -191.938(5)                      |
| $\Gamma\Gamma$ | VMC    | -191.821(2) | -191.8292(9) | -191.88(1)  | -191.93(3)                       |
| $\Gamma\Gamma$ | DMC    | -191.961(4) | -191.937(2)  | -191.940(2) | -191.943(5)                      |
| CA             | VMC    | -191.605(3) | -191.749(1)  | -191.805(1) | -191.860(2)                      |
| CA             | DMC    | -191.745(3) | -191.864(3)  | -191.909(3) | -191.954(7)                      |
| AN             | VMC    | -192.074(2) | -191.9121(9) | -191.92(1)  | -191.93(3)                       |
| AN             | DMC    | -192.211(4) | -192.004(1)  | -191.978(2) | -191.951(4)                      |

TABLE 10: QMC  $|100 \cdot \text{Kinetic}/\text{Total}|$  energies per  $n$  [Ha] for various supercell sizes.  $n$  denotes the number of  $\text{RuCl}_3$  chemical formula units in a supercell.  $[0.02, 0.005]$   $\text{Ha}^{-1}$  timestep extrapolation and T-moves were used for DMC.

| State          | Method | $n = 4$   | $n = 16$   | $n = 32$   | $\text{TDL}_{16 \rightarrow 32}$ |
|----------------|--------|-----------|------------|------------|----------------------------------|
| GS             | VMC    | 37.459(1) | 37.406(1)  | 37.443(9)  | 37.48(2)                         |
| GS             | DMC    | 37.411(2) | 37.403(2)  | 37.404(1)  | 37.406(3)                        |
| $\Gamma\Gamma$ | VMC    | 37.435(1) | 37.4005(6) | 37.441(9)  | 37.48(2)                         |
| $\Gamma\Gamma$ | DMC    | 37.389(3) | 37.396(2)  | 37.403(2)  | 37.411(4)                        |
| CA             | VMC    | 37.230(2) | 37.3283(9) | 37.3778(8) | 37.427(2)                        |
| CA             | DMC    | 37.184(2) | 37.329(2)  | 37.373(2)  | 37.417(5)                        |
| AN             | VMC    | 37.669(1) | 37.4707(6) | 37.47(1)   | 37.48(2)                         |
| AN             | DMC    | 37.621(3) | 37.4550(9) | 37.436(1)  | 37.417(3)                        |

### B. QMC Energies using PBE+ $U(1.5 \text{ eV})$ AREP Trial Wave Function

TABLE 11: QMC total energies [Ha] for various supercell sizes.  $n$  denotes the number of  $\text{RuCl}_3$  chemical formula units in a supercell.  $0.02 \text{ Ha}^{-1}$  timestep and Locality Approximation were used for DMC.

| State          | Method | $n = 4$        | $n = 16$        | $n = 32$       |
|----------------|--------|----------------|-----------------|----------------|
| GS             | VMC    | -558.30971(63) | -2233.82356(80) | -4467.4948(38) |
| GS             | DMC    | -558.92109(81) | -2235.2755(15)  | -4470.3496(24) |
| $\Gamma\Gamma$ | VMC    | -558.26444(93) | -2233.74709(70) | -4467.3898(17) |
| $\Gamma\Gamma$ | DMC    | -558.89938(62) | -2235.2122(11)  | -4470.2664(38) |
| CA             | VMC    | -558.46630(75) | -2233.98995(55) | -4467.6483(19) |
| CA             | DMC    | -559.10637(64) | -2235.45053(76) | -4470.5148(24) |
| AN             | VMC    | -558.04798(70) | -2233.56439(94) | -4467.2255(49) |
| AN             | DMC    | -558.6787(10)  | -2235.0264(12)  | -4470.0865(25) |

TABLE 12: QMC total energies per  $n$  [Ha] for various supercell sizes.  $n$  denotes the number of  $\text{RuCl}_3$  chemical formula units in a supercell.  $0.02 \text{ Ha}^{-1}$  timestep and Locality Approximation were used for DMC.

| State          | Method | $n = 4$      | $n = 16$      | $n = 32$      | $\text{TDL}_{16 \rightarrow 32}$ |
|----------------|--------|--------------|---------------|---------------|----------------------------------|
| GS             | VMC    | -139.5774(2) | -139.61397(5) | -139.6092(1)  | -139.6045(2)                     |
| GS             | DMC    | -139.7303(2) | -139.70472(9) | -139.69842(7) | -139.6921(2)                     |
| $\Gamma\Gamma$ | VMC    | -139.5661(2) | -139.60919(4) | -139.60593(5) | -139.6027(1)                     |
| $\Gamma\Gamma$ | DMC    | -139.7248(2) | -139.70076(7) | -139.6958(1)  | -139.6909(2)                     |
| CA             | VMC    | -139.6166(2) | -139.62437(3) | -139.61401(6) | -139.6036(1)                     |
| CA             | DMC    | -139.7766(2) | -139.71566(5) | -139.70359(7) | -139.6915(2)                     |
| AN             | VMC    | -139.5120(2) | -139.59777(6) | -139.6008(2)  | -139.6038(3)                     |
| AN             | DMC    | -139.6697(3) | -139.68915(7) | -139.69020(8) | -139.6913(2)                     |

TABLE 13: QMC kinetic energies per  $n$  [Ha] for various supercell sizes.  $n$  denotes the number of  $\text{RuCl}_3$  chemical formula units in a supercell.  $0.02 \text{ Ha}^{-1}$  timestep and Locality Approximation were used for DMC.

| State          | Method | $n = 4$   | $n = 16$   | $n = 32$  | $\text{TDL}_{16 \rightarrow 32}$ |
|----------------|--------|-----------|------------|-----------|----------------------------------|
| GS             | VMC    | 52.243(2) | 52.220(4)  | 52.25(2)  | 52.29(3)                         |
| GS             | DMC    | 52.246(3) | 52.2385(9) | 52.246(1) | 52.253(3)                        |
| $\Gamma\Gamma$ | VMC    | 52.240(3) | 52.215(2)  | 52.232(3) | 52.249(6)                        |
| $\Gamma\Gamma$ | DMC    | 52.239(2) | 52.233(1)  | 52.245(1) | 52.258(3)                        |
| CA             | VMC    | 51.903(2) | 52.123(2)  | 52.20(1)  | 52.27(2)                         |
| CA             | DMC    | 51.928(2) | 52.152(1)  | 52.203(1) | 52.254(3)                        |
| AN             | VMC    | 52.555(3) | 52.312(4)  | 52.30(1)  | 52.29(3)                         |
| AN             | DMC    | 52.546(3) | 52.315(2)  | 52.283(1) | 52.251(3)                        |

TABLE 14: QMC potential energies per  $n$  [Ha] for various supercell sizes.  $n$  denotes the number of  $\text{RuCl}_3$  chemical formula units in a supercell.  $0.02 \text{ Ha}^{-1}$  timestep and Locality Approximation were used for DMC.

| State          | Method | $n = 4$     | $n = 16$     | $n = 32$    | $\text{TDL}_{16 \rightarrow 32}$ |
|----------------|--------|-------------|--------------|-------------|----------------------------------|
| GS             | VMC    | -191.821(2) | -191.834(4)  | -191.86(2)  | -191.89(3)                       |
| GS             | DMC    | -191.976(3) | -191.9432(9) | -191.944(1) | -191.946(3)                      |
| $\Gamma\Gamma$ | VMC    | -191.806(3) | -191.825(2)  | -191.838(3) | -191.851(6)                      |
| $\Gamma\Gamma$ | DMC    | -191.964(2) | -191.934(1)  | -191.941(1) | -191.948(3)                      |
| CA             | VMC    | -191.520(2) | -191.748(2)  | -191.81(1)  | -191.88(2)                       |
| CA             | DMC    | -191.705(2) | -191.867(1)  | -191.907(1) | -191.946(3)                      |
| AN             | VMC    | -192.067(3) | -191.909(4)  | -191.90(1)  | -191.89(3)                       |
| AN             | DMC    | -192.215(3) | -192.004(2)  | -191.973(1) | -191.942(3)                      |

TABLE 15: QMC  $|100 \cdot \text{Kinetic/Total}|$  energies per  $n$  [Ha] for various supercell sizes.  $n$  denotes the number of  $\text{RuCl}_3$  chemical formula units in a supercell.  $0.02 \text{ Ha}^{-1}$  timestep and Locality Approximation were used for DMC.

| State          | Method | $n = 4$   | $n = 16$   | $n = 32$   | $\text{TDL}_{16 \rightarrow 32}$ |
|----------------|--------|-----------|------------|------------|----------------------------------|
| GS             | VMC    | 37.430(1) | 37.403(3)  | 37.43(1)   | 37.45(2)                         |
| GS             | DMC    | 37.391(2) | 37.3921(6) | 37.399(1)  | 37.406(2)                        |
| $\Gamma\Gamma$ | VMC    | 37.430(2) | 37.401(1)  | 37.414(2)  | 37.427(4)                        |
| $\Gamma\Gamma$ | DMC    | 37.387(1) | 37.3893(8) | 37.399(1)  | 37.409(2)                        |
| CA             | VMC    | 37.176(2) | 37.331(1)  | 37.388(9)  | 37.45(2)                         |
| CA             | DMC    | 37.151(1) | 37.3270(9) | 37.3670(9) | 37.407(2)                        |
| AN             | VMC    | 37.671(2) | 37.473(3)  | 37.463(9)  | 37.45(2)                         |
| AN             | DMC    | 37.621(2) | 37.451(1)  | 37.4276(9) | 37.404(2)                        |

### C. QMC Energies using PBE+ $U(1.5 \text{ eV})$ SOREP Trial Wave Function

TABLE 16: QMC total energies [Ha] for various supercell sizes.  $n$  denotes the number of  $\text{RuCl}_3$  chemical formula units in a supercell.  $0.02 \text{ Ha}^{-1}$  timestep and Locality Approximation were used for DMC.

| State          | Method | $n = 4$        | $n = 16$       | $n = 32$ |
|----------------|--------|----------------|----------------|----------|
| GS             | VMC    | -558.27045(89) | -2233.5595(25) |          |
| GS             | DMC    | -558.8495(12)  | -2234.9559(16) |          |
| $\Gamma\Gamma$ | VMC    | -558.2140(10)  | -2233.4801(40) |          |
| $\Gamma\Gamma$ | DMC    | -558.81387(96) | -2234.8833(18) |          |
| CA             | VMC    | -558.4314(10)  | -2233.7276(27) |          |
| CA             | DMC    | -559.03095(83) | -2235.1269(13) |          |
| AN             | VMC    | -558.01012(88) | -2233.3021(34) |          |
| AN             | DMC    | -558.60773(87) | -2234.7038(18) |          |

TABLE 17: QMC total energies per  $n$  [Ha] for various supercell sizes.  $n$  denotes the number of  $\text{RuCl}_3$  chemical formula units in a supercell.  $0.02 \text{ Ha}^{-1}$  timestep and Locality Approximation were used for DMC.

| State          | Method | $n = 4$      | $n = 16$      | $n = 32$ | TDL <sub>16→32</sub> |
|----------------|--------|--------------|---------------|----------|----------------------|
| GS             | VMC    | -139.5676(2) | -139.5975(2)  |          |                      |
| GS             | DMC    | -139.7124(3) | -139.6847(1)  |          |                      |
| $\Gamma\Gamma$ | VMC    | -139.5535(3) | -139.5925(3)  |          |                      |
| $\Gamma\Gamma$ | DMC    | -139.7035(2) | -139.6802(1)  |          |                      |
| CA             | VMC    | -139.6079(3) | -139.6080(2)  |          |                      |
| CA             | DMC    | -139.7577(2) | -139.69543(8) |          |                      |
| AN             | VMC    | -139.5025(2) | -139.5814(2)  |          |                      |
| AN             | DMC    | -139.6519(2) | -139.6690(1)  |          |                      |

TABLE 18: QMC kinetic energies per  $n$  [Ha] for various supercell sizes.  $n$  denotes the number of  $\text{RuCl}_3$  chemical formula units in a supercell.  $0.02 \text{ Ha}^{-1}$  timestep and Locality Approximation were used for DMC.

| State          | Method | $n = 4$   | $n = 16$  | $n = 32$ | TDL <sub>16→32</sub> |
|----------------|--------|-----------|-----------|----------|----------------------|
| GS             | VMC    | 52.240(3) | 52.263(9) |          |                      |
| GS             | DMC    | 52.236(3) | 52.241(3) |          |                      |
| $\Gamma\Gamma$ | VMC    | 52.232(5) | 52.26(1)  |          |                      |
| $\Gamma\Gamma$ | DMC    | 52.230(2) | 52.240(2) |          |                      |
| CA             | VMC    | 51.916(5) | 52.17(1)  |          |                      |
| CA             | DMC    | 51.934(3) | 52.157(3) |          |                      |
| AN             | VMC    | 52.541(3) | 52.352(9) |          |                      |
| AN             | DMC    | 52.538(3) | 52.320(2) |          |                      |

TABLE 19: QMC potential energies per  $n$  [Ha] for various supercell sizes.  $n$  denotes the number of  $\text{RuCl}_3$  chemical formula units in a supercell.  $0.02 \text{ Ha}^{-1}$  timestep and Locality Approximation were used for DMC.

| State          | Method | $n = 4$     | $n = 16$    | $n = 32$ | TDL <sub>16→32</sub> |
|----------------|--------|-------------|-------------|----------|----------------------|
| GS             | VMC    | -191.808(3) | -191.860(9) |          |                      |
| GS             | DMC    | -191.949(3) | -191.925(3) |          |                      |
| $\Gamma\Gamma$ | VMC    | -191.786(5) | -191.85(1)  |          |                      |
| $\Gamma\Gamma$ | DMC    | -191.934(2) | -191.920(2) |          |                      |
| CA             | VMC    | -191.524(5) | -191.78(1)  |          |                      |
| CA             | DMC    | -191.692(3) | -191.852(3) |          |                      |
| AN             | VMC    | -192.044(3) | -191.934(9) |          |                      |
| AN             | DMC    | -192.189(3) | -191.989(2) |          |                      |

TABLE 20: QMC  $|100 \cdot \text{Kinetic/Total}|$  energies per  $n$  [Ha] for various supercell sizes.  $n$  denotes the number of  $\text{RuCl}_3$  chemical formula units in a supercell.  $0.02 \text{ Ha}^{-1}$  timestep and Locality Approximation were used for DMC.

| State          | Method | $n = 4$   | $n = 16$  | $n = 32$ | TDL <sub>16→32</sub> |
|----------------|--------|-----------|-----------|----------|----------------------|
| GS             | VMC    | 37.430(2) | 37.438(7) |          |                      |
| GS             | DMC    | 37.388(2) | 37.399(2) |          |                      |
| $\Gamma\Gamma$ | VMC    | 37.428(4) | 37.436(8) |          |                      |
| $\Gamma\Gamma$ | DMC    | 37.386(2) | 37.399(1) |          |                      |
| CA             | VMC    | 37.187(4) | 37.368(8) |          |                      |
| CA             | DMC    | 37.160(2) | 37.336(2) |          |                      |
| AN             | VMC    | 37.663(2) | 37.507(7) |          |                      |
| AN             | DMC    | 37.620(2) | 37.460(1) |          |                      |

### III. COHESIVE ENERGY AND ATOMIC DATA

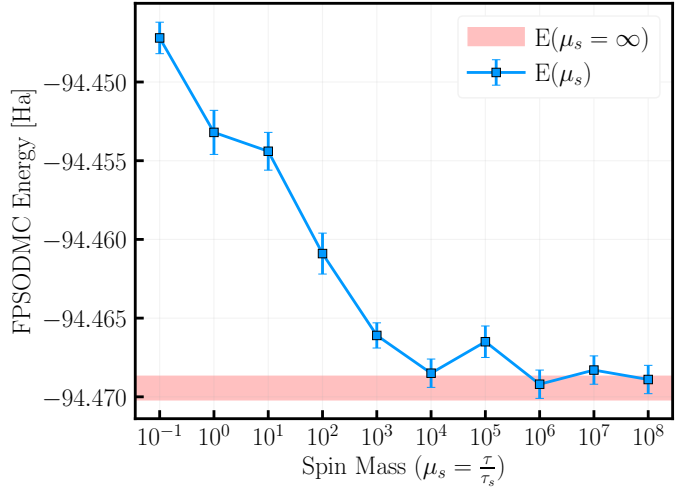

FIG. 1: Effect of spin mass on Ru atom FPSODMC energies. COSCI trial wave function is used. Spatial time step = 0.005 Ha<sup>-1</sup>.

Listing 1: reg-MDFSTU paramaters in Molpro ECP format.

```
ECP,Ru,28,4,0;
3
1, 30.000000 , 16.000000
3, 30.000000 , 480
2, 27.550000 , -156.921
2
2, 11.500590, 209.786493
2, 5.068575 , 30.214307
4
2, 10.532634, 48.751244
2, 10.192010, 97.496529
2, 4.734892 , 7.860188
2, 4.509065 , 15.329751
4
2, 8.877977 , 26.967506
2, 8.766122 , 40.432303
2, 3.170196 , 3.340758
2, 3.228851 , 5.256352
2
2, 7.820249 , -8.847525
2, 7.839647 , -11.835518
```

TABLE 21: AREP raw data is used in the calculation of cohesive energies. DMC references for isolated Ru and Cl atoms are PBE0. For atoms in boxes, the references are DFT+( $U = 1.5$ ) eV and PBE for Ru and Cl, respectively. DMC/PBE0(15%) values are timestep extrapolated and use T-Moves, while DMC/+ $U(1.5$  eV) use  $0.02 \text{ Ha}^{-1}$  timesetep with Locality Approximation.

| Method            | Ru           | Cl            | Ru_box         | Cl_box        | bulk_TDL       |
|-------------------|--------------|---------------|----------------|---------------|----------------|
| PBE               | -94.5002933  | -14.8956170   | -94.50604772   | -14.89563572  | -139.67378232  |
| PBE0(15)          | -94.4927603  | -14.8989440   | -94.49281420   | -14.89896023  | -139.64573611  |
| PBE0              | -94.4845058  | -14.9012875   | -94.48449967   | -14.90130279  | -139.63328046  |
| PBE+U1.5          |              |               | -94.49915107   | -14.89563572  | -139.62963695  |
| VMC/PBE0(15%)     | -94.4286(1)  | -14.9099(1)   |                |               | -139.60908(24) |
| DMC/PBE0(15%)     | -94.4613(2)  | -14.9192(1)   |                |               | -139.68701(20) |
| VMC/+ $U(1.5$ eV) |              |               | -94.438299(47) | -14.9118(1)   | -139.60445(24) |
| DMC/+ $U(1.5$ eV) |              |               | -94.467652(81) | -14.91981(11) | -139.69213(18) |
| RHF               | -93.80594(5) | -14.68947(1)  |                |               |                |
| Exact             | -94.4892(9)  | -14.92671(17) |                |               |                |

TABLE 22: SOREP raw data is used in the calculation of cohesive energies. DMC references for isolated Ru and Cl atoms are PBE0. For atoms in boxes, the references are DFT+( $U = 1.5$ ) eV and PBE for Ru and Cl, respectively. DMC/PBE0(15%) values are timestep extrapolated and use T-Moves, while DMC/+ $U(1.5$  eV) use  $0.02 \text{ Ha}^{-1}$  timesetep with Locality Approximation.

| Method            | Ru            | Cl            | Ru_box        | Cl_box        | bulk_TDL    |
|-------------------|---------------|---------------|---------------|---------------|-------------|
| PBE               |               | -14.8956170   | -94.515677895 | -14.89563572  | -139.683423 |
| PBE0(15)          |               | -14.8989440   |               | -14.89896023  |             |
| PBE0              |               | -14.9012875   |               | -14.90130279  |             |
| PBE+U1.5          |               |               | -94.508364    | -14.89563572  | -139.638749 |
| VMC/PBE0(15%)     | -94.4334(4)   | -14.9099(1)   |               |               |             |
| DMC/PBE0(15%)     | -94.46757(57) | -14.9192(1)   |               |               |             |
| VMC/+ $U(1.5$ eV) |               |               | -94.43092(33) | -14.9118(1)   |             |
| DMC/+ $U(1.5$ eV) |               |               | -94.46530(13) | -14.91981(11) |             |
| RHF               | -93.81909666  | -14.68947(1)  |               |               |             |
| Exact             |               | -14.92671(17) |               |               |             |

#### IV. NODAL SURFACE OPTIMIZATION

TABLE 23: QMC/PBE0( $w$ ) total energies [Ha] for various exact exchange factors  $w$ . FN-DMC timestep 0.02 Ha<sup>-1</sup>. Conventional cell ( $n = 4$  RuCl<sub>3</sub> units). ZZ phase. AVG is the average of all tabulated states.

| PBE0( $\omega$ [%]) | GS(VMC)      | GS(DMC)      | $\Gamma\Gamma$ (VMC) | $\Gamma\Gamma$ (DMC) | CA(VMC)      | CA(DMC)      | AN(VMC)      | AN(DMC)      | AVG(VMC)     | AVG(DMC)     |
|---------------------|--------------|--------------|----------------------|----------------------|--------------|--------------|--------------|--------------|--------------|--------------|
| PBE                 | -558.236(1)  | -558.8655(7) | -558.251(1)          | -558.8749(8)         | -558.434(2)  | -559.0700(8) | -558.016(2)  | -558.6473(7) | -558.2344(7) | -558.8644(4) |
| PBE0(5)             | -558.2850(7) | -558.891(1)  | -558.262(1)          | -558.874(1)          | -558.450(1)  | -559.079(1)  | -558.0488(6) | -558.660(1)  | -558.2615(4) | -558.8763(5) |
| PBE0(10)            | -558.3199(8) | -558.900(2)  | -558.2813(7)         | -558.880(1)          | -558.4769(7) | -559.084(2)  | -558.0640(8) | -558.663(1)  | -558.2856(4) | -558.8815(7) |
| PBE0(15)            | -558.3398(7) | -558.9066(8) | -558.290(1)          | -558.8827(9)         | -558.495(1)  | -559.0904(8) | -558.0758(6) | -558.666(1)  | -558.3001(5) | -558.8865(5) |
| PBE0(20)            | -558.351(1)  | -558.908(1)  | -558.2976(7)         | -558.8804(8)         | -558.5032(7) | -559.090(1)  | -558.0826(7) | -558.665(1)  | -558.3087(4) | -558.8859(6) |
| PBE0(25)            | -558.3560(6) | -558.908(1)  | -558.2672(6)         | -558.862(1)          | -558.5100(6) | -559.086(1)  | -558.0872(8) | -558.6648(9) | -558.3051(3) | -558.8802(5) |
| PBE0(30)            | -558.361(1)  | -558.904(1)  | -558.2675(6)         | -558.8563(9)         | -558.5127(7) | -559.082(1)  | -558.0882(9) | -558.660(1)  | -558.3075(4) | -558.8757(6) |

TABLE 24: QMC/PBE+ $U_{eff}$  total energies [Ha] various  $U_{eff}$  values. FN-DMC timestep 0.02 Ha<sup>-1</sup>. Conventional cell ( $n = 4$  RuCl<sub>3</sub> units). ZZ phase. AVG is the average of all tabulated states.

| $U_{eff}$ [eV] | GS(VMC)     | GS(DMC)      | $\Gamma\Gamma$ (VMC) | $\Gamma\Gamma$ (DMC) | CA(VMC)     | CA(DMC)      | AN(VMC)     | AN(DMC)      | AVG(VMC)     | AVG(DMC)     |
|----------------|-------------|--------------|----------------------|----------------------|-------------|--------------|-------------|--------------|--------------|--------------|
| 0.00           | -558.239(2) | -558.8647(8) | -558.250(1)          | -558.8758(7)         | -558.436(1) | -559.0705(6) | -558.014(2) | -558.6466(6) | -558.2349(7) | -558.8644(4) |
| 0.50           | -558.265(1) | -558.8762(8) | -558.245(2)          | -558.8691(7)         | -558.428(2) | -559.0680(8) | -558.029(2) | -558.6497(8) | -558.2420(8) | -558.8658(4) |
| 1.00           | -558.291(2) | -558.8892(7) | -558.2599(9)         | -558.8732(7)         | -558.452(1) | -559.0776(9) | -558.042(1) | -558.6551(8) | -558.2614(6) | -558.8738(4) |
| 1.50           | -558.309(1) | -558.8966(8) | -558.2654(9)         | -558.8757(7)         | -558.466(1) | -559.0830(7) | -558.047(2) | -558.657(1)  | -558.2718(7) | -558.8780(4) |
| 2.50           | -558.327(2) | -558.9038(8) | -558.241(1)          | -558.859(1)          | -558.486(2) | -559.0860(8) | -558.059(1) | -558.6609(8) | -558.2780(8) | -558.8773(4) |
| 3.00           | -558.331(1) | -558.9041(8) | -558.237(2)          | -558.8558(7)         | -558.486(1) | -559.0835(7) | -558.059(1) | -558.660(1)  | -558.2783(6) | -558.8759(4) |

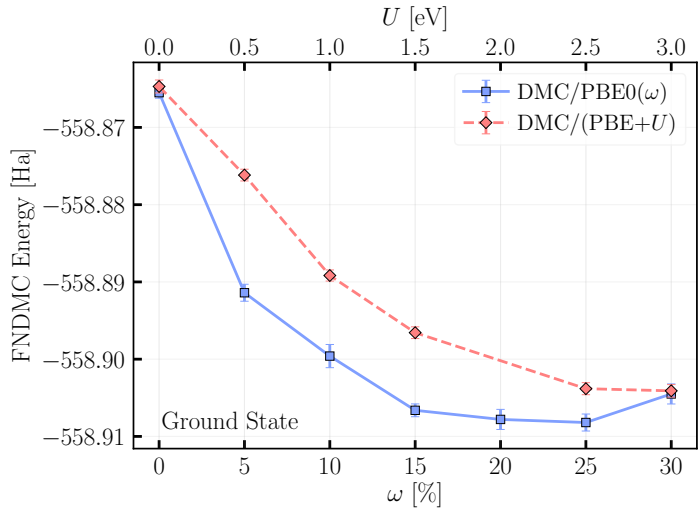

(a)

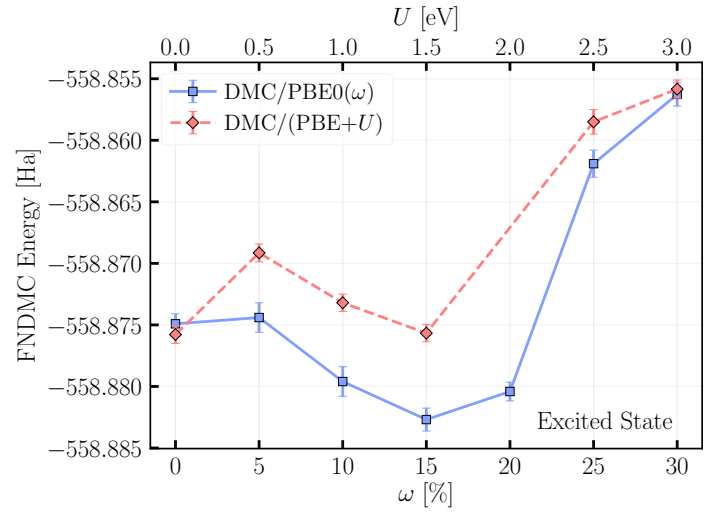

(b)

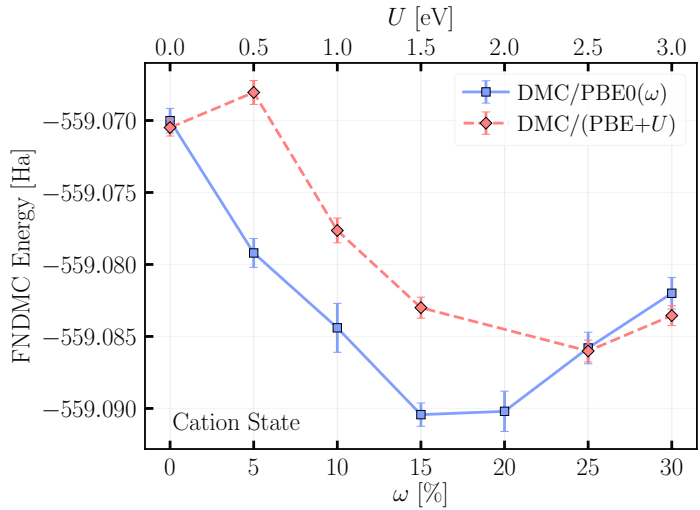

(c)

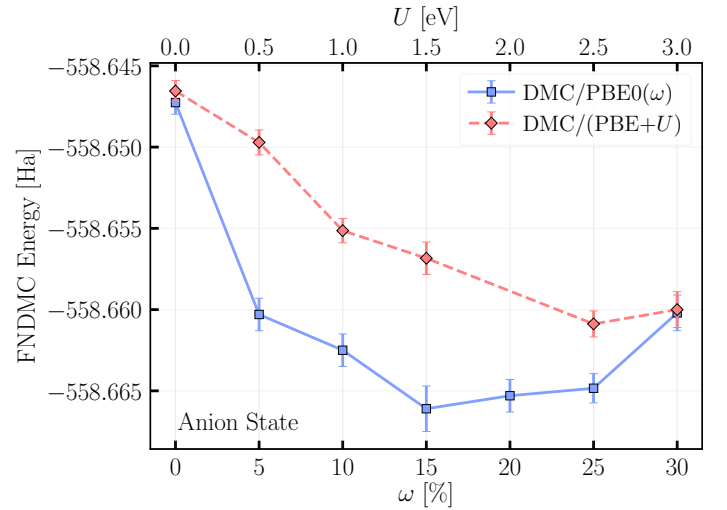

(d)

FIG. 2: FN-DMC calculations for various nodal surfaces using exact exchange factor  $\omega$  and Hubbard  $U_{eff}$ . FN-DMC timestep 0.02 Ha<sup>-1</sup>. Conventional cell ( $n = 4$  RuCl<sub>3</sub> units). ZZ phase. (a) Ground state, (b)  $\Gamma \rightarrow \Gamma$  excited state, (c) cation state, (d) anion state,

## V. QMC SUPERCELLS

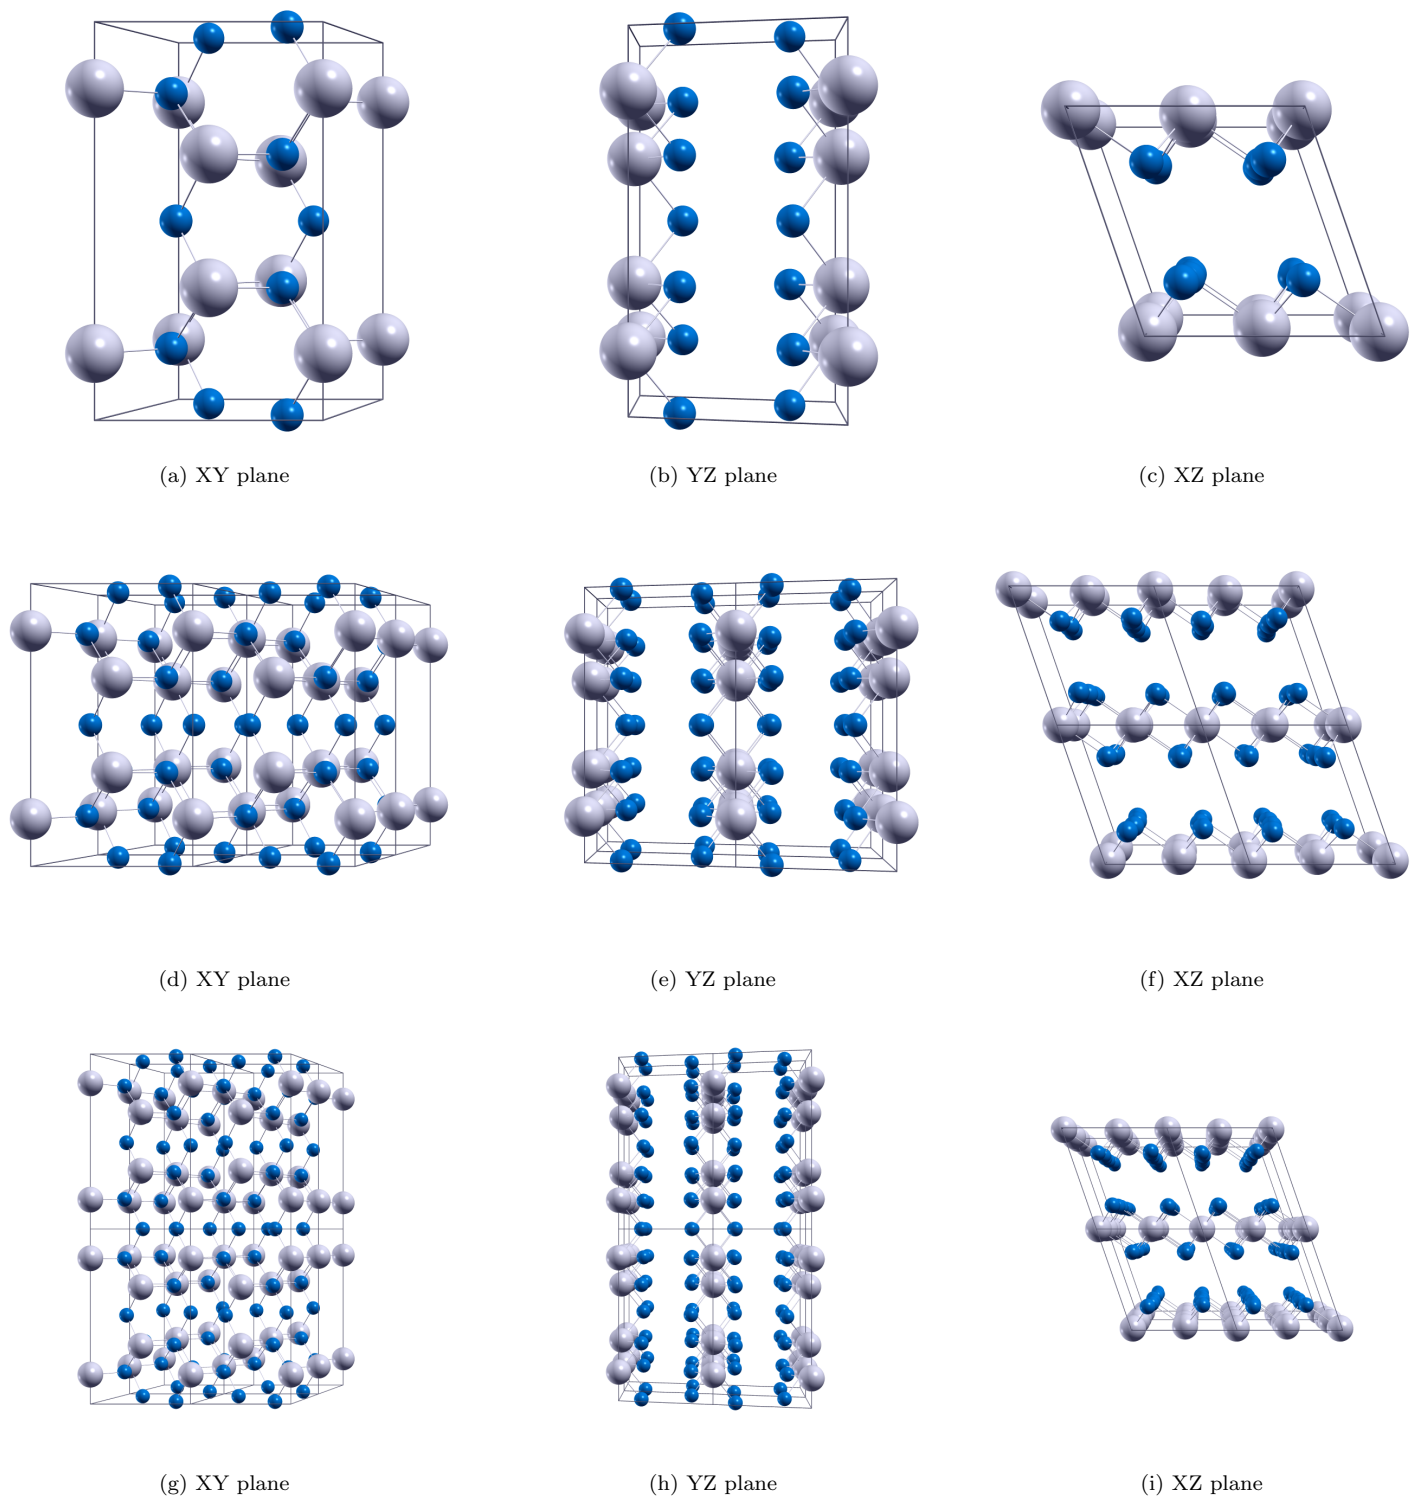

FIG. 3: Illustrations of various supercells employed in this work. Large spheres with light colors are Ru atoms, and small spheres with dark colors are Cl atoms. Top row:  $1 \times 1 \times 1$  ( $xyz$ ) of conventional cell,  $n = 4$   $\text{RuCl}_3$  units. Middle row:  $2 \times 1 \times 2$  ( $xyz$ ) of conventional cell,  $n = 16$   $\text{RuCl}_3$  units. Bottom row:  $2 \times 2 \times 2$  ( $xyz$ ) of conventional cell,  $n = 32$   $\text{RuCl}_3$  units.

## VI. GEOMETRY AND SYMMETRY

TABLE 25: The geometry and crystal symmetry from [1].

| Space Group               | C2/m              |         |
|---------------------------|-------------------|---------|
| Lattice<br>Parameters     | a (Å)             | 5.9230  |
|                           | b (Å)             | 10.3291 |
|                           | c (Å)             | 6.011   |
|                           | $\beta$           | 109.14° |
| Fractional<br>Coordinates | Ru <sub>1</sub> x | 0.0000  |
|                           | Ru <sub>1</sub> y | 0.1677  |
|                           | Ru <sub>1</sub> z | 0.0000  |
|                           | Cl <sub>1</sub> x | 0.2300  |
|                           | Cl <sub>1</sub> y | 0.0000  |
|                           | Cl <sub>1</sub> z | 0.2340  |
|                           | Cl <sub>2</sub> x | 0.2492  |
|                           | Cl <sub>2</sub> y | 0.1718  |
|                           | Cl <sub>2</sub> z | -0.2337 |

The geometry and crystal symmetry used in this work is obtained from experimental values [1].

---

[1] A. Banerjee, C. A. Bridges, J.-Q. Yan, A. A. Aczel, L. Li, M. B. Stone, G. E. Granroth, M. D. Lumsden, Y. Yiu, J. Knolle, S. Bhattacharjee, D. L. Kovrizhin, R. Moessner, D. A. Tennant,

D. G. Mandrus, and S. E. Nagler, Nature Materials **15**, 733 (2016).
